# Supplementary material for: Improving the Regularity of Vector Fields
Source: arXiv:2105.10120 source file (2022-05-22)
Supplement: Supplementary file 1 [file appendix.tex]

\section{Another Space for Differential Forms Along Vector Fields}

In this section, we investigate more on the properties of $\Co^\beta_{X,\loc}$-objects especially when $X=(X_1,\dots,X_q)$ is a very rough collection of vector fields. In particular, we will Proposition \ref{Prop::FuncVF::ZygVF=Zyg} \ref{Item::FuncVF::ZygVF=Zyg::dForms}, \ref{Item::FuncVF::ZygVF=Zyg::Cor} and \ref{Item::FuncVF::ZygVF=Zyg::Diff} without assuming $\alpha\ge1$.

We introduce a different space of differential forms along $X=(X_1,\dots,X_q)$. Unlike the Definition \ref{Defn::FuncVf::formregularity} that requires $\alpha>\frac12$, the following definition makes sense even when $\alpha\in(0,\frac12]$.
\begin{defn}\label{Defn::FuncRevisVF::TildeZygVF}
Let $\alpha>0$ and let $X_1,\dots,X_q$ be $\Co^\alpha$-vector fields defined on a $\Co^{\alpha+1}$-manifold $\Manifold$. Let $\beta>-\alpha$ and let $1\le k\le n$, we define $\ZygVF\beta X(\Manifold;\mywedge^kT^*\Manifold)$ recursively as follows:
\begin{itemize}
    \item $\beta\in(-\alpha,0]$, $\ZygVF\beta X(\Manifold;\mywedge^kT^*\Manifold):=\Co^\beta_{\loc}(\Manifold;\mywedge^kT^*\Manifold)$.
    \item $\beta\in(0,1]$, $\ZygVF\beta X(\Manifold;\mywedge^kT^*\Manifold)$ consist of continuous form $\theta\in C^0_\loc(\Manifold;\mywedge^kT^*\Manifold)$ such that $d\IntProd{X_1}\theta,\dots,d\IntProd{X_q}\theta$ have regularity $\Co^{\beta-1}_\loc(\Manifold)$.
    \item $\beta>1$, $\ZygVF\beta X(\Manifold;\mywedge^kT^*\Manifold)$ consist of $\theta\in \ZygVF{\beta-1} X(\Manifold;\mywedge^kT^*\Manifold)$ such that $\theta,d\IntProd{X_1}\theta,\dots,d\IntProd{X_q}\theta\in\ZygVF{\beta-1} X(\Manifold;T^*\Manifold)$.
\end{itemize}
\end{defn}
\begin{rmk}\label{Rmk::FuncRevisVF::RmkForTildeZygVF}
\begin{enumerate}[(i)]
    \item\label{Item::FuncRevisVF:RmkForTildeZygVF::HasandTilde} When $\beta>1-\alpha$, the statement $d\theta\in\ZygVF{\beta-1}X(\Manifold;\mywedge^kT^*\Manifold)$ is equivalent to $d\theta$ having regularity $\Co^{\beta-1}_{X,\loc}(\Manifold)$ (see Definition \ref{Defn::FuncVf::RegularityofForms}).
    \item When $\alpha>\frac12$ and $\beta>\alpha$, $\ZygVF\beta X(\Manifold;\mywedge^kT^*\Manifold)$ and $\Co^\beta_{X,\loc}(\Manifold;\mywedge^kT^*\Manifold)$ may not coincide. See Example \ref{Example::ZygVFvsTildeZygVF}. This is due to the fact that $\omega\in\ZygVF\beta X\not\Rightarrow d\omega\in\ZygVF{\beta-1}X$. Nevertheless they coincide for exact differential forms. See Proposition \ref{Prop::FuncRevisVF::ZygVF=Zyg::Form} \ref{Item::FuncRevisVF::ZygVF=Zyg::Form::3}.
\end{enumerate}
\end{rmk}

\section{A Schauder's Estimate of Second Order Elliptic}\label{Section::AppendixSchauder}
In this part, we prove Lemma \ref{Lemma::FuncRevisVF::SchauderEstimate}. 

Recall from Lemma \ref{Lemma::FuncSpace::Product} the map $(f,g)\mapsto\nabla^2(fg)$ is a continuous map $\Co^\beta(\Ball^n)\to\Co^\alpha(\Ball^n)\to\Co^{\beta-2}(\Ball^n;\Mbb^{n\times n})$ for all $\alpha>0$ and $\beta\in(-\alpha,\alpha]$. Recall from Lemma \ref{Lemma::FuncRevis::NewtonianBoundedness}, $[f\mapsto\Green\ast f]:\Co^{\beta-2}_c(\Ball^n)\to\Co^\beta(\Ball^n)$ is a norm-bounded linear map for all $\beta\in\R$, where $\Green$ is the Newtonian potential given in \eqref{Eqn::FuncRevis::GreensFunction}. Therefore, given $\alpha,\beta>0$ there is a $C=C_{n,\alpha,\beta}>0$ such that
\begin{equation}\label{Eqn::AppendixSchauder::Bounded}
    \|\chi\left(\Green\ast\nabla^2(fg))\right)\|_{\Co^\beta(\Ball^n;\Mbb^{n\times n})}\le C_{n,\alpha,\beta}\|\chi\|_{\Co^\alpha(\Ball^n)}\|f\|_{\Co^\beta(\Ball^n)}\|g\|_{\Co^\alpha(\Ball^n)},\quad\forall f,\chi\in\Co^\beta_c(\Ball^n),g\in\Co^\alpha(\Ball^n).
\end{equation}

We are going to choose $c$ in Lemma \ref{Lemma::FuncRevisVF::SchauderEstimate} based on \eqref{Eqn::AppendixSchauder::Bounded}.
\begin{proof}[Proof of Lemma \ref{Lemma::FuncRevisVF::SchauderEstimate}]
Fix $\alpha,\eps>0$ and $\beta\in(-\alpha,\alpha]$. Recall $(\Dc^gu)_i=\sum_{k,l=1}^n\partial_{kl}^2(g_i^{klj}u_j)$ is a second order differential operator with $g_i^{klj}\in\Co^\alpha_\loc(\Ball^n)$. Since the operator is symmetric to the indices $k$ and $l$, replacing $g_i^{klj}$ by $\frac12(g_i^{klj}+g_i^{lkj})$ we can assume that $g_i^{klj}=g_i^{lkj}$.

Let $N\in\Z_+$ be the smallest integer such that $\eps-\alpha+N>\beta$. We fix $\chi^{-1},\chi^0,\dots,\chi^N\in C_c^\infty(\Ball^n)$ such that $\chi^r\equiv1$ in a neighborhood of $0$ for all $r=-1,\dots,N$ and $\supp\chi^{r+1}\Subset\{x:\chi^r(x)=1\}^\circ$ for $r=0,\dots,N$. We choose 
\begin{equation}\label{Eqn::AppendixSchauder::Tmp0}
    c=\left(m^2n^2\cdot\max\left(C_{n,\alpha,\eps-\alpha}\|\chi^{-1}\|_{\Co^\alpha},C_{n,\alpha,\eps-\alpha+1}\|\chi^0\|_{\Co^\alpha},\dots,C_{n,\alpha,\eps-\alpha+N-1}\|\chi^{N-2}\|_{\Co^\alpha},C_{n,\alpha,\beta})\|\chi^{N-1}\|_{\Co^\alpha}\right)\right)^{-1}.
\end{equation} Here $C_{n,\alpha,\gamma}$ is the constant in \eqref{Eqn::AppendixSchauder::Bounded}. We claim that $c>0$ is the small constant that we need.

For $r=0,\dots,N-1$, define Banach space $\Xs^r$ as the completion of $\Co^{\eps-\alpha+r}_c(\Ball^n;\R^m)$ under $\Co^{\eps-\alpha+r}$-norm, and define $\Xs^N $ as the completion of $\Co^\beta_c(\Ball^n;\R^m)$ under $\Co^\beta$-norm.

Now assume $\sum_{i,j=1}^m\sum_{k,l=1}^n\|g_i^{klj}\|_{\Co^\alpha(\Ball^n)}<c$. So the choice of $c$ in \eqref{Eqn::AppendixSchauder::Tmp0} indicates that
\begin{equation}\label{Eqn::AppendixSchauder::Contractions}
    [\phi\mapsto\chi^{r-1}(\Green\ast\Delta\phi)]:\Xs^r\to\Xs^r\text{ and }[\phi\mapsto\chi^{r-1}\Green\ast\Delta\phi]:\Xs^{r+1}\to\Xs^{r+1}\text{ are contractions},\quad r=0,\dots,N-1,
\end{equation}

Now assume $u\in\Co^{\eps-\alpha}_\loc(\Ball^n;\R^m)$ satisfies $\Delta u+\Dc^gu\in\Co^{\beta-2}_\loc(\Ball^n;\R^m)$.
We denote $v^r=\chi^ru$ and $f^r=\Delta v^r+\Dc^gv^r$ for $r=0,\dots,N$ so $v^r=\chi^rv^{r-1}$ when $r\ge1$. We use induction to show that $v^r\in\Co^{\eps-\alpha+r}(\Ball^n;\R^m)$ for $r=0,\dots,N-1$ and $v^N\in\Co^\beta(\Ball^n;\R^m)$. Since $v^N=\chi^Nu$ equals to $u$ near the origin, we then conclude the proof.

Suppose $v^{r}\in\Co^{\eps-\alpha+r}(\Ball^n;\R^m)$ holds, we wish to prove $v^{r+1}\in\Co^{\eps-\alpha+r+1}(\Ball^n;\R^m)$. Note that the base case $r=0$ is true because $v^0=\chi^0u\in\Co^{\eps-\alpha}(\Ball^n;\R^m)$ based on the assumption.

Now $v^{r+1}=\chi^{r+1}v^r$ satisfies the following equation:
\begin{equation}\label{Eqn::AppendixSchauder::Tmp1}
    \Delta v^{r+1}=\Delta(\chi^{r+1} v^r)=\chi^{r+1}\Delta v^r+2\nabla\chi^{r+1}\cdot\nabla v^r+(\Delta\chi^{r+1})v^r=(\chi^{r+1}f^r-\chi^{r+1}\Dc^gv^r)+2\nabla\chi^{r+1}\cdot\nabla v^r+(\Delta\chi^{r+1})v^r.
\end{equation}

Write $v^r=(v^r_1,\dots,v^r_m)$ and $f^r=(f^r_1,\dots,f^r_m)$, so for $i=1,\dots,m$,
\begin{equation}\label{Eqn::AppendixSchauder::Tmp2}
    (\chi^{r+1}\Dc^gv^r)_i=\sum_{k,l=1}^n\sum_{j=1}^m\chi^{r+1}\partial_{kl}^2(g_i^{klj}v^r_j)=\sum_{k,l=1}^n\sum_{j=1}^m\left(\partial_{kl}^2(g_i^{klj}\chi^{r+1}v^r_j)-v^r_j\partial^2_{kl}(g_i^{klj}\chi^{r+1})-2\partial_kv^r_j\partial_l(g_i^{klj}\chi^{r+1})\right).
\end{equation}

Combining \eqref{Eqn::AppendixSchauder::Tmp1} and \eqref{Eqn::AppendixSchauder::Tmp2}, we have, for $i=1,\dots,m$,
\begin{equation}\label{Eqn::AppendixSchauder::Tmp3}
\begin{aligned}
     \Delta v^{r+1}_i&=-\sum_{k,l=1}^n\sum_{j=1}^m\partial^2_{kl}(g_i^{klj}v^{r+1}_j)+\chi^{r+1}f^r_i+\sum_{k,l=1}^n\sum_{j=1}^m\left(v^r_j\partial^2_{kl}\left((g_i^{klj}-\delta^{kl}\delta_i^j)\chi^{r+1}\right)+2\partial_kv^r_j\partial_l\left((g_i^{klj}-\delta^{kl}\delta_i^j)\chi^{r+1}\right)\right)
     \\
     &=:-\sum_{k,l=1}^n\sum_{j=1}^m\partial^2_{kl}(g_i^{klj}v^{r+1}_j)+h^r_i=(\Dc^gv^{r+1})_i+h^r_i.
\end{aligned}
\end{equation}
By induction hypothesis $v^r\in\Co_c^{\eps-\alpha+r}(\Ball^n;\R^m)\subsetneq\Xs^r$, so from \eqref{Eqn::AppendixSchauder::Tmp3} we see that $h^r=(h^r_i)_{i=1}^m\in\Co_c^{\min(\eps-\alpha+r-2,\beta-2)}(\Ball^n;\R^m)$ (that is $h^r\in \Co_c^{\eps-\alpha+r-2}$ when $r<N$ and $h^r\in\Co_c^{\beta-2}$ when $r=N$).

Note that $\Green\ast\Delta v^{r+1}$ is defined and $(\Green\ast\Delta v^{r+1})\big|_{\partial\Ball^n}\in C^\infty(\overline{\Ball^n};\R^m)$ because $v^{r+1}$ has compact support. So $v^{r+1}-\Green\ast\Delta v^{r+1}\in C^\infty(\overline{\Ball^n};\R^m)$ since it is harmonic function. Recall that $\Xs^{r+1}$ is the Banach space given by the completion of $\Co_c^{\min(\eps-\alpha+r+1,\beta)}(\Ball^n;\R^m)$ under $\Co^{\min(\eps-\alpha+r+1,\beta)}$-norm. Note that $v^{r+1}-\Green \ast\Delta v^{r+1}+\Green\ast h^r\in\Co_c^{\min(\eps-\alpha+r+1,\beta)}(\Ball^n;\R^m)$ implies $\chi^{r-1}(v^{r+1}-\Green \ast\Delta v^{r+1}+\Green\ast h^r)\in\Xs^{r+1}$.

Now we see that $v^{r+1}=\chi^{r-1}v^{r+1}=\chi^{r-1}(v^{r+1}-\Green \ast\Delta v^{r+1})+\chi^{r-1}(\Green \ast\Delta v^{r+1})$ is a fixed point of $\phi\in\Xs^r$ to the equation
\begin{equation}\label{Eqn::AppendixSchauder::Tmp4}
    \phi=\chi^{r-1}(v^{r+1}-\Green \ast\Delta v^{r+1}+\Green\ast h^r)+\chi^{r-1}(\Green\ast\Dc^g\phi).
\end{equation}
Note that \eqref{Eqn::AppendixSchauder::Tmp4} is an affine linear equation, and note that the right hand side of \eqref{Eqn::AppendixSchauder::Tmp4} is in $\Xs^{r+1}$ if $\phi\in\Xs^{r+1}$. While by \eqref{Eqn::AppendixSchauder::Contractions} $[\phi\mapsto\chi^{r-1}(\Green\ast\Dc^g\phi)]$ is contraction map in both $\Xs^r$ and $\Xs^{r+1}$. So by Banach fixed point theorem $v^{r+1}$ is the unique fixed point to the equation \eqref{Eqn::AppendixSchauder::Tmp4} in both $\Xs^r$ and $\Xs^{r+1}$, which means $v^{r+1}\in\Co_c^{\eps-\alpha+r+1}(\Ball^n;\R^m)$ if $r<N-1$ and $v^{r+1}\in\Co_c^{\beta}(\Ball^n;\R^m)$ if $r=N-1$. Therefore, we complete the induction process and finish the proof.
\end{proof}
